# Supplementary material for: CBench: Towards Better Evaluation of Question Answering Over Knowledge Graphs
Source: arXiv:2105.00811 source file (2021-04-05)
Supplement: Supplementary file 1 [file Appendix_QuestionAnalysisTables.tex]

**\appendix
\section{Results of Natural Language Question Analysis}
\input{Results of Natural Language Question Analysis}

%\clearpage% Flush earlier floats (otherwise order might not be correct)

    \begin{landscape}% Landscape page
    \begin{scriptsize}
    \centering
          \begin{table}
           
        \setlength{\tabcolsep}{3pt} %% default is 6pt
        \begin{tabular}{|l|ll|ll|ll|ll|ll|ll|ll|ll|ll|ll|ll|ll|}
\hline
	 & \multicolumn{2}{l}{QALD 1}  & \multicolumn{2}{l}{QALD 2}  & \multicolumn{2}{l}{QALD 3}  & \multicolumn{2}{l}{QALD 4}  & \multicolumn{2}{l}{QALD 5}  & \multicolumn{2}{l}{QALD 6}  & \multicolumn{2}{l}{QALD 7}  & \multicolumn{2}{l}{QALD 8}  & \multicolumn{2}{l}{QALD 9}  & \multicolumn{2}{l}{QALD ALL}  & \multicolumn{2}{l}{LC-QUAD}  & \multicolumn{2}{l}{FREEBASE}  \\ \hline
	 & A\# & R\% & A\# & R\% & A\# & R\% & A\# & R\% & A\# & R\% & A\# & R\% & A\# & R\% & A\# & R\% & A\# & R\% & A\# & R\% & A\# & R\% & A\# & R\% \\ \hline
	Wh-Questions & 124 & 62.3 & 187 & 54.3 & 220 & 55.4 & 201 & 62.6 & 200 & 59.9 & 273 & 63.3 & 347 & 65.5 & 207 & 65.7 & 255 & 62.5 & 723 & 62.0 & 42077 & 89.0 & 8955 & 81.6 \\ 
	How-Questions & 21 & 10.6 & 44 & 12.8 & 53 & 13.3 & 25 & 7.8 & 35 & 10.5 & 45 & 10.4 & 61 & 11.5 & 41 & 13.0 & 44 & 10.8 & 147 & 12.6 & 595 & 1.3 & 500 & 4.5 \\
	Yes/No Questions & 19 & 9.5 & 34 & 9.9 & 36 & 9.1 & 24 & 7.5 & 26 & 7.8 & 30 & 7.0 & 55 & 10.4 & 33 & 10.5 & 37 & 9.1 & 89 & 7.6 & 1000 & 2.1 & 9 & 0.1 \\ 
	Requests & 35 & 17.6 & 78 & 22.7 & 87 & 21.9 & 68 & 21.2 & 71 & 21.2 & 81 & 18.8 & 59 & 11.1 & 34 & 10.8 & 72 & 17.6 & 197 & 16.9 & 2662 & 5.6 & 513 & 4.7 \\ 
	Topicalized Questions & 0 & 0 & 1 & 0.3 & 1 & 0.3 & 3 & 0.9 & 2 & 0.6 & 2 & 0.5 & 8 & 1.5 & 0 & 0 & 0 & 0 & 11 & 0.9 & 939 & 2.0 & 999 & 9.1 \\ \hline
\end{tabular}
\captionof{table}{Question count by type for each benchmark. A\# is the absolute value and R\% is the relative value.}% Add 'table' caption
          \label{table:type}
        \end{table}
        
        \centering
        \begin{table}
        \setlength{\tabcolsep}{3pt} %% default is 6pt
        \begin{tabular}{|l|l|l|l|l|l|l|l|l|l|l|l|l|}
\hline
	 & QALD 1  & QALD 2  & QALD 3  & QALD 4  & QALD 5  & QALD 6  & QALD 7  & QALD 8  & QALD 9 & QALD-ALL  & LC-QUAD  & FREEBASE  \\ \hline
	What & 13 & 21 & 29 & 34 & 37 & 60 & 62 & 57 & 55 & 126 & 25221 & 4917 \\ 
	When & 19 & 22 & 27 & 10 & 12 & 18 & 27 & 15 & 14 & 70 & 0 & 242 \\
	Where & 1 & 2 & 2 & 3 & 6 & 10 & 12 & 8 & 12 & 22 & 4668 & 1134 \\ 
	Which & 63 & 92 & 101 & 115 & 92 & 112 & 141 & 66 & 105 & 318 & 6247 & 1047 \\ 
	Who, whose, whom & 28 & 50 & 61 & 39 & 53 & 73 & 105 & 61 & 69 & 187 & 5918 & 1608 \\ \hline
\end{tabular}
\captionof{table}{Wh-question count for each benchmark}% Add 'table' caption
          \label{table:upos}
        \end{table}
        
        \centering
        \begin{table}
        \setlength{\tabcolsep}{3pt} %% default is 6pt
        \begin{tabular}{|l|l|l|l|l|l|l|l|l|l|l|l|l|}
\hline
	 & QALD 1  & QALD 2  & QALD 3  & QALD 4  & QALD 5  & QALD 6  & QALD 7  & QALD 8  & QALD 9 & QALD-ALL  & LC-QUAD  & FREEBASE  \\ \hline
	Cluster 1 & 23 & 28 & 27 & 26 & 23 & 21 & 22 & 18 & 21 & 23 & 18 & 19 \\ 
	Cluster 2 & 21 & 19 & 20 & 20 & 22 & 22 & 22 & 26 & 23 & 20 & 32 & 26 \\
	Cluster 3 & 3 & 4 & 3 & 10 & 3 & 3 & 9 & 4 & 3 & 6 & 9 & 8 \\ 
	Cluster 4 & 23 & 22 & 21 & 17 & 18 & 19 & 17 & 17 & 18 & 21 & 19 & 25 \\ 
	Cluster 5 & 30 & 27 & 29 & 27 & 34 & 35 & 30 & 35 & 35 & 30 & 22 & 22 \\ \hline
\end{tabular}
\captionof{table}{Question distribution (\%) clustered based on UPOS for each benchmark}% Add 'table' caption
          \label{table:upos}
        \end{table}
        
        \centering
        \begin{table}
        \setlength{\tabcolsep}{3pt} %% default is 6pt
        \begin{tabular}{|l|l|l|l|l|l|l|l|l|l|l|l|l|}
\hline
	 &QALD 1  & QALD 2  & QALD 3  & QALD 4  & QALD 5  & QALD 6  & QALD 7  & QALD 8  & QALD 9 & QALD-ALL  & LC-QUAD  & FREEBASE  \\ \hline
	Cluster 1 & 27 & 26 & 28 & 22 & 27 & 28 & 26 & 28 & 27 & 25 & 25 & 31 \\ 
	Cluster 2 & 2 & 4 & 4 & 9 & 5 & 5 & 12 & 7 & 5 & 8 & 15 & 10 \\
	Cluster 3 & 18 & 17 & 18 & 13 & 19 & 19 & 21 & 26 & 22 & 19 & 20 & 14 \\ 
	Cluster 4 & 11 & 9 & 7 & 10 & 9 & 11 & 13 & 15 & 12 & 10 & 32 & 21 \\ 
	Cluster 5 & 42 & 44 & 43 & 46 & 40 & 37 & 28 & 24 & 34 & 38 & 8 & 24 \\ \hline
\end{tabular}
\captionof{table}{Question distribution (\%) clustered based on Detailed tags for each benchmark}% Add 'table' caption
        \label{table:detailed}
        \end{table}
        
        \centering
        \begin{table}
        \setlength{\tabcolsep}{3pt} %% default is 6pt
        \begin{tabular}{|l|l|l|l|l|l|l|l|l|l|l|l|l|}
\hline
	 & QALD 1  & QALD 2  & QALD 3  & QALD 4  & QALD 5  & QALD 6  & QALD 7  & QALD 8  & QALD 9 & QALD-ALL  & LC-QUAD  & FREEBASE  \\ \hline
	Cluster 1 & 26 & 22 & 23 & 19 & 21 & 23 & 19 & 23 & 22 & 21 & 17 & 20 \\ 
	Cluster 2 & 19 & 17 & 19 & 14 & 18 & 19 & 17 & 19 & 19& 18 & 17 & 17 \\
	Cluster 3 & 29 & 29 & 27 & 27 & 28 & 26 & 24 & 26 & 27 & 24 & 20 & 24 \\ 
	Cluster 4 & 12 & 11 & 12 & 14 & 17 & 17 & 16 & 16 & 16 & 14 & 31 & 15 \\ 
	Cluster 5 & 14 & 21 & 19 & 26 & 16 & 15 & 24 & 16 & 16 & 23 & 15 & 24 \\ \hline
\end{tabular}
\captionof{table}{Question distribution (\%) clustered based on Dependency Parse Tree for each benchmark}% Add 'table' caption
          \label{table:parse}
        \end{table}  
        
    \end{scriptsize}
    \end{landscape}
%\clearpage% Flush page
