# Supplementary material for: CBench: Towards Better Evaluation of Question Answering Over Knowledge Graphs
Source: arXiv:2105.00811 source file (2021-04-05)
Supplement: Supplementary file 2 [file Appendix_QAGraph.tex]

\section{Question Answering Systems Summary Graph}
\label{app:qa_graph}
