# Supplementary material for: CBench: Towards Better Evaluation of Question Answering Over Knowledge Graphs
Source: arXiv:2105.00811 source file (2021-04-05)
Supplement: Supplementary file 3 [file Appendix_Question_Analysis.tex]

\section{Question Analysis Experiment Design}
\label{app:qAnalysis}
